# Supplementary material for: Are Retrials All You Need? Enhancing Large Language Model Reasoning Without Verbalized Feedback
Source: arXiv:2504.12951 source file (2025-04-17)
Supplement: Supplementary file 1 [file additional_imports.tex]

\RequirePackage{algorithm}
\RequirePackage{algorithmic}
\usepackage{tikz}
\usepackage{subfig}
\usetikzlibrary{calc, shapes, positioning, arrows.meta, fit}

\usepackage{amsmath}

\usepackage{listings}

% Define a comment command
\usepackage{comment}
\newcommand{\blockcomment}[1]{}

\definecolor{codegreen}{rgb}{0,0.6,0}
\definecolor{codegray}{rgb}{0.5,0.5,0.5}
\definecolor{codepurple}{rgb}{0.58,0,0.82}
\definecolor{backcolour}{rgb}{0.95,0.95,0.92}

\lstdefinestyle{mystyle}{
    backgroundcolor=\color{backcolour},   
    commentstyle=\color{codegreen},
    keywordstyle=\color{magenta},
    numberstyle=\tiny\color{codegray},
    stringstyle=\color{codepurple},
    basicstyle=\ttfamily\footnotesize,
    breakatwhitespace=false,         
    breaklines=true,                 
    captionpos=b,                    
    keepspaces=true,                 
    numbers=left,                    
    numbersep=5pt,                  
    showspaces=false,                
    showstringspaces=false,
    showtabs=false,                  
    tabsize=2
}

\lstset{style=mystyle}
